# Supplementary material for: Broken adiabaticity induced by Lifshitz transition in MoS$_2$ and WS$_2$ single layers
Source: arXiv:1907.04766 ancillary file (2020-01-28)
Supplement: Supplementary file 1 [file SuppInfo.pdf]

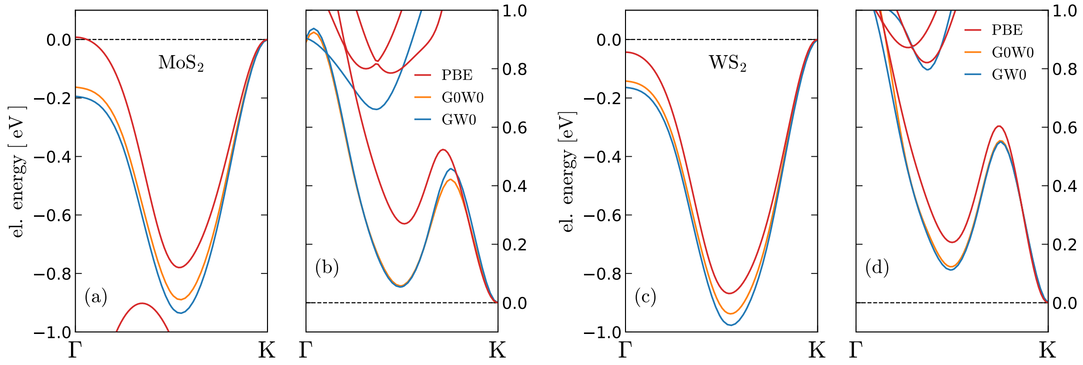


**Supplementary Figure 1**. (a) Valence and (b) conduction bands of $MoS_2$ single layer as obtained with the PBE [1] functional as well as with G0W0 and self-consistent GW0 approaches [2] (without spin-orbit coupling). (c),(d) Same as in (a) and (b) but for $WS_2$ single layer.

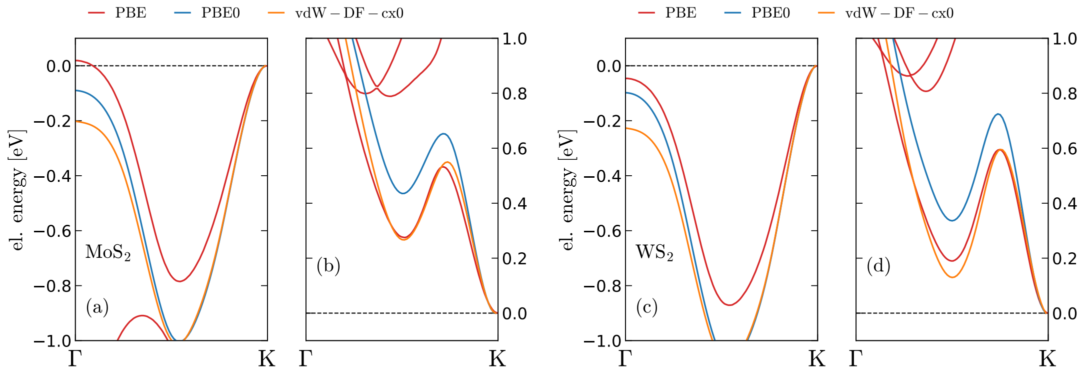


**Supplementary Figure 2**. (a) Valence and (b) conduction bands of $MoS_2$ single layer as obtained with the PBE and hybrid functionals (i.e., PBE0 [3] and vdW-DF-cx0 [4]). Spin-orbit coupling is not included. (c),(d) Same as in (a) and (b) but for $WS_2$ single layer.

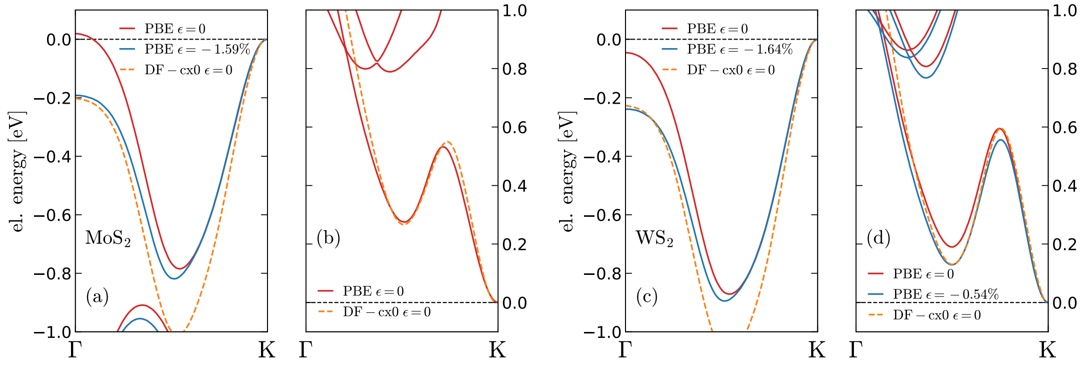


**Supplementary Figure 3**. (a) Valence and (b) conduction bands of $MoS_2$ single layer as obtained with the PBE functional with relaxed unit cell ($\epsilon = 0$), with the PBE functional and strained unit cell ($\epsilon = -1.59\%$ for valence band), and with the vdW-DF-cx0 hybrid functional. The right amount of strain is applied in order to recreate the right band topology as obtained with hybrid functional. Spin-orbit coupling is not included. (c),(d) Same as in (a) and (b) but for $WS_2$ single layer. Here, the strains $\epsilon = -1.64\%$ and $\epsilon = -0.54\%$ are used in order to simulate the right topology of the valence and conduction bands, respectively.

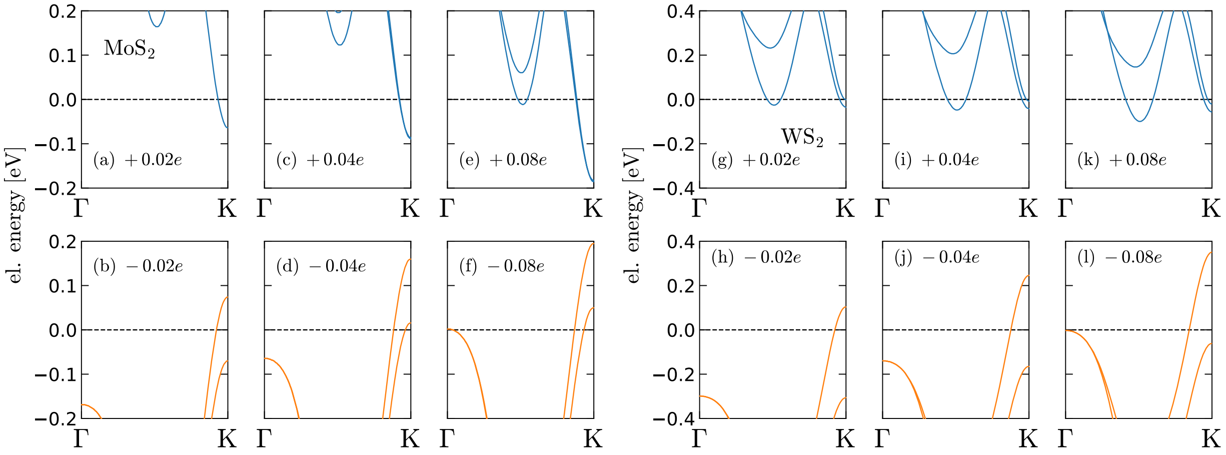


**Supplementary Figure 4**. Final electronic band structures for doped TMDs obtained with PBE+SOC used in the main part of the manuscript, where the corresponding unit cell parameters were modified in order to obtain the right topology of the conduction and valence bands (i.e., as obtained with DF-cx0 functional). (a)-(f) and (g)-(l) panels show the conduction and valence bands for $MoS_2$ and $WS_2$, respectively. The dopings $\pm 0.02e$, $\pm 0.04e$, and $\pm 0.08e$ correspond to carrier densities of $\pm 2.34 \cdot 10^{13}\,\mathrm{cm}^{-2}$, $\pm 4.69 \cdot 10^{13}\,\mathrm{cm}^{-2}$, and $\pm 9.38 \cdot 10^{13}\,\mathrm{cm}^{-2}$, respectively.

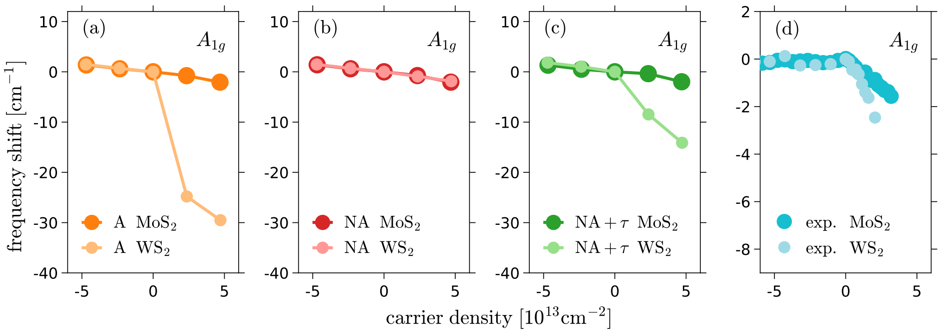


**Supplementary Figure 5**. Phonon frequency shifts of the $A_{1g}$ mode as obtained with (a) the adiabatic (A) approximation, with (b) inclusion of nonadiabatic corrections (NA), and in addition with (c) electron-hole pairs scattering due to EPC (NA + $\tau$). The theoretical results are compared with (d) the experimental data extracted from Ref. [5].

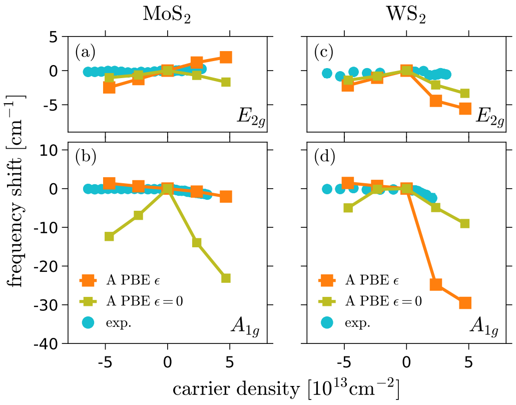


**Supplementary Figure 6**. Comparison between the different adiabatic (A) phonon frequency shifts for the $E_{2g}$ and $A_{1g}$ modes of (a)-(b) $MoS_2$ and (c)-(d) $WS_2$ as a function of doping when the relaxed PBE structures (with the wrong valley topology) are used and when the strained structures are used that recreate the right topology of the bands. The experimental results from Ref. [5] are also shown.

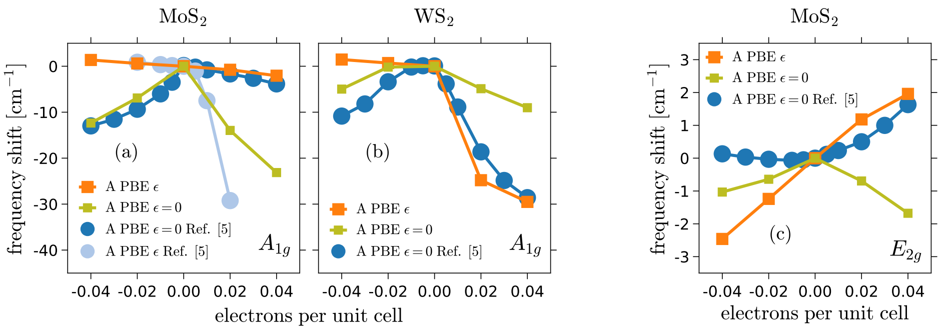


**Supplementary Figure 7**. Comparison between the present results shown in Supplementary Figure 6 with the adiabatic (A) results from Ref. [5] for the (a) $A_{1g}$ and (c) $E_{2g}$ modes of $MoS_2$ and for (b) the $A_{1g}$ mode of $WS_2$. Some discrepancy is present, however it mostly comes from the fact that here different unit cell parameters were used for hole and electron dopings in order to capture the right topology of valence and conduction bands. For example, the final adiabatic results from this work (orange squares) compares very good with the original PBE results of Ref. [5] for electron dopings and with the strained PBE results of Ref. [5] for hole dopings.

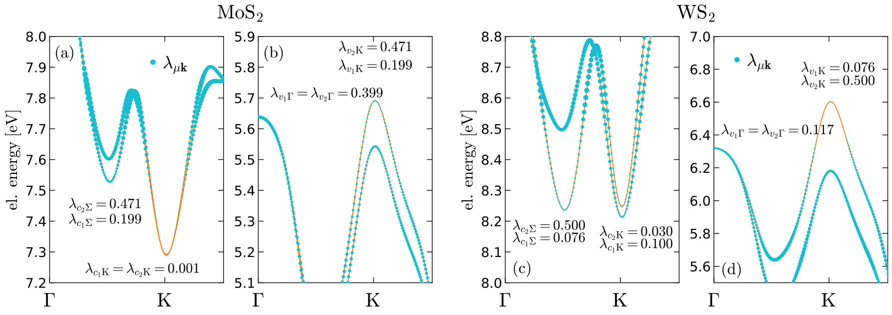


**Supplementary Figure 8**. Electron band- and momentum-resolved electron-phonon coupling constants $\lambda_{\mu\mathbf{k}}$ for conduction and valence bands of (a)-(b) $MoS_2$ and (c)-(d) $WS_2$. The electron band- and momentum-resolved electron-phonon coupling constant is defined as $\lambda_{\mu\mathbf{k}} = \mathrm{Im}\,\Sigma_{\mu\mathbf{k}}(\varepsilon_{\mu\mathbf{k}})/\pi k_B T$, where $\Sigma_{\mu\mathbf{k}}(\omega)$ is the standard Fan-Migdal electron self-energy [6]. The latter quantities were obtained by means of EPW using the $(48 \times 48 \times 1)$ phonon momentum grid. In both systems, drastically different EPC were obtained in two valence valleys. In the case of $MoS_2$ it turns out that EPC in the Σ valley is much stronger than in the K valley.

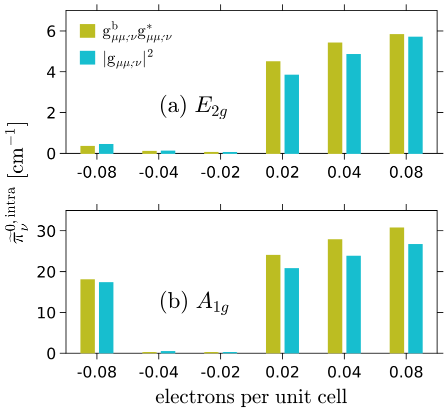


**Supplementary Figure 9**. Intraband nonadiabatic phonon self-energy $\widetilde{\pi}^{0,\mathrm{intra}}_\nu(\omega)$ obtained with $g^b_{\mu\mu',\nu} g^*_{\mu\mu',\nu}$ and $|g_{\mu\mu',\nu}|^2$ for the (a) $E_{2g}$ and (b) $A_{1g}$ phonon modes in the case of doped $WS_2$. The phonon self-energies $\widetilde{\pi}^{0,\mathrm{intra}}_\nu(\omega)$ with $|g_{\mu\mu',\nu}|^2$ were calculated with the personally modified version of the EPW code [7], while the corresponding input quantities (electron energies, phonon frequencies, and electron-phonon coupling elements) were interpolated using maximally localized Wannier functions [8]. The $\mathbf{k}$ summations in the latter phonon self-energies were done on a $(480 \times 480 \times 1)$ grid.

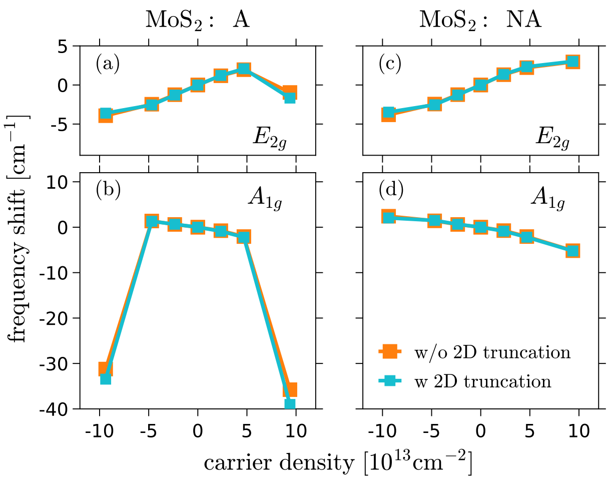


**Supplementary Figure 10**. (a)-(b) Adiabatic (A) and (c)-(d) nonadiabatic (NA) phonon frequency shifts for $MoS_2$ obtained in the present paper without and with 2D Coulomb interaction truncation, which eliminates the spurious interaction between periodic images (i.e., layers) [9, 10]. However, no significant difference between the two types of calculations were obtained.

**Supplementary Note 1. Intraband nonadiabatic phonon self-energy**

The bare nonadiabatic (dynamical) phonon self-enery $\widetilde{\pi}^0_\nu(\mathbf{q},\omega)$ (i.e., without electron-hole scattering processes) is defined as the difference between the full $\pi^0_\nu(\mathbf{q},\omega)$ and adiabatic $\pi^0_\nu(\mathbf{q},0)$ phonon self-energies [6], i.e.,

$$\widetilde{\pi}^0_\nu(\mathbf{q},\omega) \equiv \pi^0_\nu(\mathbf{q},\omega) - \pi^0_\nu(\mathbf{q},0) = \sum_{\mu\mu'\mathbf{k}} g^b_{\mu\mu',\nu}(\mathbf{k},\mathbf{q}) g^*_{\mu\mu',\nu}(\mathbf{k},\mathbf{q},\omega) \frac{f(\varepsilon_{\mu\mathbf{k}}) - f(\varepsilon_{\mu'\mathbf{k}+\mathbf{q}})}{\omega + i\eta + \varepsilon_{\mu\mathbf{k}} - \varepsilon_{\mu'\mathbf{k}+\mathbf{q}}} - \sum_{\mu\mu'\mathbf{k}} g^b_{\mu\mu',\nu}(\mathbf{k},\mathbf{q}) g^*_{\mu\mu',\nu}(\mathbf{k},\mathbf{q},0) \frac{f(\varepsilon_{\mu\mathbf{k}}) - f(\varepsilon_{\mu'\mathbf{k}+\mathbf{q}})}{\varepsilon_{\mu\mathbf{k}} - \varepsilon_{\mu'\mathbf{k}+\mathbf{q}}} \quad \text{(S1)}$$

where the dynamically screened and bare electron-phonon coupling functions are defined as $g_{\mu\mu',\nu}(\mathbf{k},\mathbf{q},\omega) = \langle\psi_{\mu\mathbf{k}}|\,\Delta_{\mathbf{q}\nu}V_{\mathrm{scf}}(\omega)\,|\psi_{\mu'\mathbf{k}+\mathbf{q}}\rangle/\sqrt{2M\omega_{\mathrm{A}}}$ and $g^b_{\mu\mu',\nu}(\mathbf{k},\mathbf{q}) = \langle\psi_{\mu\mathbf{k}}|\,\Delta_{\mathbf{q}\nu}V_{\mathrm{ion}}\,|\psi_{\mu'\mathbf{k}+\mathbf{q}}\rangle/\sqrt{2M\omega_{\mathrm{A}}}$, respectively. The self-consistent potential is $\Delta_{\mathbf{q}\nu}V_{\mathrm{scf}}(\mathbf{r},\omega) = \Delta_{\mathbf{q}\nu}V_{\mathrm{ion}}(\mathbf{r}) + \int d\mathbf{r}' K(\mathbf{r},\mathbf{r}')\Delta_{\mathbf{q}\nu}n(\mathbf{r}',\omega)$ [where $K(\mathbf{r},\mathbf{r}') = \delta E_{Hxc}[n]/\delta n(\mathbf{r})\delta n(\mathbf{r}')$]. Note that the dynamical screening is usually approximated with the static one, i.e., $\Delta_{\mathbf{q}\nu}V_{\mathrm{scf}}(\omega) \to \Delta_{\mathbf{q}\nu}V_{\mathrm{scf}}(0)$ [6, 11]. The relevant contribution for simulating the Raman spectra is the long-wavelength part ($\mathbf{q} \approx \mathbf{0}$), and the corresponding interband and intraband parts of the full and adiabatic phonon self-energies have the following forms

$$\begin{aligned}
\pi^{0,\mathrm{inter}}_\nu(\mathbf{q}\approx 0,\omega) &= \sum_{\mu\neq\mu'\mathbf{k}} g^b_{\mu\mu',\nu}(\mathbf{k},0) g^*_{\mu\mu',\nu}(\mathbf{k},0,\omega) \frac{f(\varepsilon_{\mu\mathbf{k}}) - f(\varepsilon_{\mu'\mathbf{k}})}{\omega + i\eta + \varepsilon_{\mu\mathbf{k}} - \varepsilon_{\mu'\mathbf{k}}}, \\
\pi^{0,\mathrm{intra}}_\nu(\mathbf{q}\approx 0,\omega) &= 0, \\
\pi^{0,\mathrm{inter}}_\nu(\mathbf{q}\approx 0,0) &= \sum_{\mu\neq\mu'\mathbf{k}} g^b_{\mu\mu',\nu}(\mathbf{k},0) g^*_{\mu\mu',\nu}(\mathbf{k},0,0) \frac{f(\varepsilon_{\mu\mathbf{k}}) - f(\varepsilon_{\mu'\mathbf{k}})}{\varepsilon_{\mu\mathbf{k}} - \varepsilon_{\mu'\mathbf{k}}}, \\
\pi^{0,\mathrm{intra}}_\nu(\mathbf{q}\approx 0,0) &= \sum_{\mu\mathbf{k}} g^b_{\mu\mu,\nu}(\mathbf{k},0) g^*_{\mu\mu,\nu}(\mathbf{k},0,0) \frac{\partial f(\varepsilon_{\mu\mathbf{k}})}{\partial\varepsilon_{\mu\mathbf{k}}}.
\end{aligned} \quad \text{(S2)}$$

Under the assumption of $\Delta_{\mathbf{q}\nu}V_{\rm scf}(\omega)\to\Delta_{\mathbf{q}\nu}V_{\rm scf}(0)$, the final expression for the nonadiabatic $\mathbf{q}\approx\mathbf{0}$ phonon self-energy turns out to be

$$\widetilde{\pi}^0_\nu(\omega)\equiv\widetilde{\pi}^0_\nu(\mathbf{q}\approx 0,\omega)=\sum_{\mu\neq\mu'\mathbf{k}}\frac{\omega|g_{\mu\mu',\nu}(\mathbf{k},0,0)|^2}{\varepsilon_{\mu'\mathbf{k}}-\varepsilon_{\mu\mathbf{k}}}\frac{f(\varepsilon_{\mu\mathbf{k}})-f(\varepsilon_{\mu'\mathbf{k}})}{\omega+i\eta+\varepsilon_{\mu\mathbf{k}}-\varepsilon_{\mu'\mathbf{k}}} +\sum_{\mu\mathbf{k}}g^b_{\mu\mu,\nu}(\mathbf{k},0)g^*_{\mu\mu,\nu}(\mathbf{k},0,0)\left[-\frac{\partial f(\varepsilon_{\mu\mathbf{k}})}{\partial\varepsilon_{\mu\mathbf{k}}}\right], \tag{S3}$$

Note that the equivalence $g^b_{\mu\mu',\nu}g^*_{\mu\mu',\nu}=|g_{\mu\mu',\nu}|^2$ holds in the interband part of $\widetilde{\pi}^0_\nu(\omega)$ when static screening is assumed in $\pi^{0,\rm inter}_\nu(\mathbf{q}\approx 0,\omega)$, because the exchange and correlation part of $\Delta_{\mathbf{q}\nu}V_{\rm scf}(0)$ is then equal in $\pi^{0,\rm inter}_\nu(\mathbf{q}\approx 0,\omega)$ and $\pi^{0,\rm inter}_\nu(\mathbf{q}\approx 0,0)$ [12]. However, this is not true for the intraband part of $\widetilde{\pi}^0_\nu(\omega)$ since $\pi^{0,\rm intra}_\nu(\mathbf{q}\approx 0,\omega)$ is zero and thus there is no equivalent cancelation.

The interband phonon self-energy is negligible for semiconducting transition metal dichalcogenides since the characteristic phonon energies are much smaller than the energies of the interband transitions, i.e., $\omega\ll|\varepsilon_{\mu\mathbf{k}}-\varepsilon_{\mu'\mathbf{k}}|$, (see Supplementary Table **2**) and thus the only dynamical correction to the adiabatic phonon energies comes from the intraband part [i.e., from the second term in Eq. (S3)]. The nonadiabatic correction to the phonon energy is then

$$\omega^2-\omega_{\rm A}^2=2\omega_{\rm A}\widetilde{\pi}^{0,\rm intra}_\nu(\omega), \tag{S4}$$

or

$$\omega-\omega_A\approx\widetilde{\pi}^{0,\rm intra}_\nu(\omega). \tag{S5}$$

The standard treatment of Eqs. (S1) and (S3) is to approximate the bare vertex function with the screened one, i.e., $g^b_{\mu\mu',\nu}g^*_{\mu\mu',\nu}\to|g_{\mu\mu',\nu}|^2$ [6, 13–15]. A more exact approach would be to estimate the bare vertex by unscreening $g_{\mu\mu',\nu}$, i.e., $g^b_{\mu\mu',\nu}=\epsilon_{\rm M}g_{\mu\mu',\nu}$, where $\epsilon_{\rm M}$ is the macroscopic dielectric function [11].

Here I introduce an another approach that is applicable only for the intraband phonon self-energy in the $\mathbf{q}\approx 0$ limit. Namely, the $\mathbf{q}\approx 0$ dynamical matrix in the adiabatic DFPT contains exactly this intraband term but with the opposite sign. Thus one can use the standard DFPT approach to isolate the nonadibatic intraband term. The dynamical matrix at $\mathbf{q}\approx 0$ is defined as

$$\mathcal{D}(\omega)\equiv\mathcal{D}(\mathbf{q}\approx 0,\omega)=\int d\mathbf{r}\Delta n(\mathbf{r},\omega)|_{\mathbf{q}\approx 0}\Delta V_{\rm ion}(\mathbf{r})+\int d\mathbf{r}n(\mathbf{r})\Delta^2V_{\rm ion}(\mathbf{r}), \tag{S6}$$

where the perturbation of the charge density with the displacement has the following form within the linear response

$$\Delta n(\mathbf{r},\omega)|_{\mathbf{q}\approx 0}=\sum_{\mu\mu'\mathbf{k}}\frac{[f(\varepsilon_{\mu\mathbf{k}})-f(\varepsilon_{\mu'\mathbf{k}})]d^*_{\mu\mu',\nu}(\mathbf{k},0,\omega)}{\omega+i\eta+\varepsilon_{\mu\mathbf{k}}-\varepsilon_{\mu'\mathbf{k}}}\psi^*_{\mu\mathbf{k}}(\mathbf{r})\psi_{\mu'\mathbf{k}}(\mathbf{r}). \tag{S7}$$

The screened deformation potential is defined as $d^*_{\mu\mu',\nu}(\mathbf{k},\mathbf{q},\omega)=\langle\psi_{\mu'\mathbf{k}+\mathbf{q}}|\,\Delta_{\mathbf{q}\nu}V_{\rm scf}(\mathbf{r},\omega)\,|\psi_{\mu\mathbf{k}}\rangle$. By introducing Eq. (S7) into Eq. (S6), the force constant matrix bacomes

$$\mathcal{D}(\omega)=\sum_{\mu\mu'\mathbf{k}}\frac{[f(\varepsilon_{\mu\mathbf{k}})-f(\varepsilon_{\mu'\mathbf{k}})]d^*_{\mu\mu',\nu}(\mathbf{k},0,\omega)d^b_{\mu\mu',\nu}(\mathbf{k},0)}{\omega+i\eta+\varepsilon_{\mu\mathbf{k}}-\varepsilon_{\mu'\mathbf{k}}}+\int d\mathbf{r}n(\mathbf{r})\Delta^2V_{\rm ion}(\mathbf{r}), \tag{S8}$$

where $d^b_{\mu\mu',\nu}(\mathbf{k},\mathbf{q})=\langle\psi_{\mu\mathbf{k}+\mathbf{q}}|\,\Delta_{\mathbf{q}\nu}V_{\rm ion}(\mathbf{r})\,|\psi_{\mu\mathbf{k}}\rangle$ is the bare deformation potential. Note that Eq. (S8) is usually expressed in the form where $d^b_{\mu\mu',\nu}(\mathbf{k},0)$ is replaced with $d_{\mu\mu',\nu}(\mathbf{k},0,\omega)$ by using the following equation $\Delta V_{\rm ion}(\mathbf{r})=\Delta V_{\rm scf}(\mathbf{r},\omega)-\int d\mathbf{r}'K(\mathbf{r},\mathbf{r}')\Delta n(\mathbf{r}',\omega)$, e.g., see Eqs. (4) and (5) in Ref. [15]. In the standard DFPT approach, the

(adiabatic) phonon energies $\omega_\mathrm{A}$ are then obtained with $\omega_\mathrm{A}^2 = \mathcal{D}(0)/M$, i.e.,

$$\omega_\mathrm{A}^2 = \frac{1}{M}\sum_{\mu\neq\mu'\mathbf{k}} d^*_{\mu\mu',\nu}(\mathbf{k},0,0)d^b_{\mu\mu',\nu}(\mathbf{k},0)\frac{f(\varepsilon_{\mu\mathbf{k}})-f(\varepsilon_{\mu'\mathbf{k}})}{\varepsilon_{\mu\mathbf{k}}-\varepsilon_{\mu'\mathbf{k}}} + \frac{1}{M}\sum_{\mu\mathbf{k}} d^*_{\mu\mu,\nu}(\mathbf{k},0,0)d^b_{\mu\mu,\nu}(\mathbf{k},0)\frac{\partial f(\varepsilon_{\mu\mathbf{k}})}{\partial\varepsilon_{\mu\mathbf{k}}} + \frac{1}{M}\int d\mathbf{r}n(\mathbf{r})\Delta^2 V_\mathrm{ion}(\mathbf{r}). \tag{S9}$$

Now it is possible to exclude the intraband part of the dynamical matrix by removing the relevant intraband transitions from the Sternheimer equation of the linear response [16]. Such procedure for calculating partially renormalized phonon energies, which include the screening effects coming from reduced number of electronic transitions, is described in Ref. [17]. The partially renormalized adiabatic phonon energy for which the intraband transitions are removed is

$$(\omega_\mathrm{A}^{(p)})^2 = \frac{1}{M}\sum_{\mu\neq\mu'\mathbf{k}} d^*_{\mu\mu',\nu}(\mathbf{k},0,0)d^b_{\mu\mu',\nu}(\mathbf{k},0)\frac{f(\varepsilon_{\mu\mathbf{k}})-f(\varepsilon_{\mu'\mathbf{k}})}{\varepsilon_{\mu\mathbf{k}}-\varepsilon_{\mu'\mathbf{k}}} + \frac{1}{M}\int d\mathbf{r}n(\mathbf{r})\Delta^2 V_\mathrm{ion}(\mathbf{r}). \tag{S10}$$

And then finally by subtracting fully [Eq. (S9)] from partially [Eq. (S10)] renormalized adiabatic phonon energy one gets

$$(\omega_\mathrm{A}^{(p)})^2 - \omega_\mathrm{A}^2 = -\frac{1}{M}\sum_{\mu\mathbf{k}} d^*_{\mu\mu,\nu}(\mathbf{k},0,0)d^b_{\mu\mu,\nu}(\mathbf{k},0)\frac{\partial f(\varepsilon_{\mu\mathbf{k}})}{\partial\varepsilon_{\mu\mathbf{k}}}, \tag{S11}$$

or

$$\omega_\mathrm{A}^{(p)} - \omega_\mathrm{A} \approx -\frac{1}{2M\omega_\mathrm{A}}\sum_{\mu\mathbf{k}} d^*_{\mu\mu,\nu}(\mathbf{k},0,0)d^b_{\mu\mu,\nu}(\mathbf{k},0)\frac{\partial f(\varepsilon_{\mu\mathbf{k}})}{\partial\varepsilon_{\mu\mathbf{k}}}, \tag{S12}$$

which exactly corresponds to the nonadiabatic intraband phonon self-energy $\widetilde{\pi}_\nu^{0,\mathrm{intra}}(\omega)$.

In Supplementary Figure **9** the difference between the phonon self-energies $\widetilde{\pi}_\nu^{0,\mathrm{intra}}(\omega)$ obtained with $g^b_{\mu\mu',\nu}g^*_{\mu\mu',\nu}$ and $|g_{\mu\mu',\nu}|^2$ is shown for doped $WS_2$ and for $E_{2g}$ and $A_{1g}$ modes.

**Supplementary Table 1**. Absolute adiabatic frequencies of $E_{2g}$ and $A_{1g}$ modes for relaxed and strained structures, which are used in order to recreate the right topology of the bands. These values are used as reference points in Figures 1 and 2 of the main text.

| | $MoS_2$ | | $WS_2$ | | |
|---|---|---|---|---|---|
| | $\epsilon = 0$ | $\epsilon = -1.59\%$ | $\epsilon = 0$ | $\epsilon = -1.64\%$ | $\epsilon = -0.54\%$ |
| $\omega^\mathrm{A}_{E_{2g}}$ [cm$^{-1}$] | 373.2 | 380.4 | 342.7 | 349.0 | 344.9 |
| $\omega^\mathrm{A}_{A_{1g}}$ [cm$^{-1}$] | 396.4 | 398.7 | 405.2 | 407.9 | 406.1 |

**Supplementary Table 2**. Intraband and interband contributions to the bare nonadiabatic phonon self-energy [see Eq. (S3)] for the $E_{2g}$ and $A_{1g}$ phonon modes of $MoS_2$ and for different charge dopings. All the values of phonon self-energies are in cm$^{-1}$.

| | | electrons per unit cell | | | | | |
|---|---|---|---|---|---|---|---|
| | | −0.08 | −0.04 | −0.02 | 0.02 | 0.04 | 0.08 |
| $MoS_2$, $\nu = E_{2g}$ | $\widetilde{\pi}_\nu^{0,\mathrm{intra}}$ [cm$^{-1}$] | 0.114 | 0.021 | 0.005 | 0.140 | 0.26 | 3.912 |
| | Re $\widetilde{\pi}_\nu^{0,\mathrm{inter}}$ [cm$^{-1}$] | −0.017 | −0.017 | −0.017 | −0.017 | −0.017 | −0.017 |
| | Im $\widetilde{\pi}_\nu^{0,\mathrm{inter}}$ [cm$^{-1}$] | 0.011 | 0.011 | 0.011 | 0.011 | 0.011 | 0.011 |
| $MoS_2$, $\nu = A_{1g}$ | $\widetilde{\pi}_\nu^{0,\mathrm{intra}}$ [cm$^{-1}$] | 33.648 | 0.035 | 0.000 | 0.0165 | 0.003 | 30.598 |
| | Re $\widetilde{\pi}_\nu^{0,\mathrm{inter}}$ [cm$^{-1}$] | −0.008 | −0.010 | −0.010 | −0.009 | −0.010 | −0.012 |
| | Im $\widetilde{\pi}_\nu^{0,\mathrm{inter}}$ [cm$^{-1}$] | 0.005 | 0.006 | 0.006 | 0.006 | 0.006 | 0.008 |

## Supplementary References


[1] John P. Perdew, Kieron Burke, and Matthias Ernzerhof, "Generalized gradient approximation made simple," Phys. Rev. Lett. **77**, 3865–3868 (1996).

[2] Falco Hüser, Thomas Olsen, and Kristian S. Thygesen, "Quasiparticle gw calculations for solids, molecules, and two-dimensional materials," Phys. Rev. B **87**, 235132 (2013).

[3] John P. Perdew, Matthias Ernzerhof, and Kieron Burke, "Rationale for mixing exact exchange with density functional approximations," The Journal of Chemical Physics **105**, 9982 (1996).

[4] Kristian Berland, Yang Jiao, Jung-Hoon Lee, Tonatiuh Rangel, Jeffrey B. Neaton, and Per Hyldgaard, "Assessment of two hybrid van der waals density functionals for covalent and non-covalent binding of molecules," The Journal of Chemical Physics **146**, 234106 (2017).

[5] Thibault Sohier, Evgeniy Ponomarev, Marco Gibertini, Helmuth Berger, Nicola Marzari, Nicolas Ubrig, and Alberto F. Morpurgo, "Enhanced electron-phonon interaction in multivalley materials," Phys. Rev. X **9**, 031019 (2019).

[6] Feliciano Giustino, "Electron-phonon interactions from first principles," Rev. Mod. Phys. **89**, 015003 (2017).

[7] S. Poncé, E.R. Margine, C. Verdi, and F. Giustino, "Epw: Electronphonon coupling, transport and superconducting properties using maximally localized wannier functions," Computer Physics Communications **209**, 116 (2016).

[8] Nicola Marzari, Arash A. Mostofi, Jonathan R. Yates, Ivo Souza, and David Vanderbilt, "Maximally localized wannier functions: Theory and applications," Rev. Mod. Phys. **84**, 1419 (2012).

[9] Thibault Sohier, Matteo Calandra, and Francesco Mauri, "Two-dimensional fröhlich interaction in transition-metal dichalcogenide monolayers: Theoretical modeling and first-principles calculations," Phys. Rev. B **94**, 085415 (2016).

[10] Thibault Sohier, Matteo Calandra, and Francesco Mauri, "Density functional perturbation theory for gated two-dimensional heterostructures: Theoretical developments and application to flexural phonons in graphene," Phys. Rev. B **96**, 075448 (2017).

[11] Fabio Caruso, Moritz Hoesch, Philipp Achatz, Jorge Serrano, Michael Krisch, Etienne Bustarret, and Feliciano Giustino, "Nonadiabatic kohn anomaly in heavily boron-doped diamond," Phys. Rev. Lett. **119**, 017001 (2017).

[12] Matteo Calandra, Gianni Profeta, and Francesco Mauri, "Adiabatic and nonadiabatic phonon dispersion in a wannier function approach," Phys. Rev. B **82**, 165111 (2010).

[13] Dino Novko, "Nonadiabatic coupling effects in $mgb_2$ reexamined," Phys. Rev. B **98**, 041112 (2018).

[14] A. Marco Saitta, Michele Lazzeri, Matteo Calandra, and Francesco Mauri, "Giant nonadiabatic effects in layer metals: Raman spectra of intercalated graphite explained," Phys. Rev. Lett. **100**, 226401 (2008).

[15] Michele Lazzeri and Francesco Mauri, "Nonadiabatic kohn anomaly in a doped graphene monolayer," Phys. Rev. Lett. **97**, 266407 (2006).

[16] Stefano Baroni, Stefano de Gironcoli, Andrea Dal Corso, and Paolo Giannozzi, "Phonons and related crystal properties from density-functional perturbation theory," Rev. Mod. Phys. **73**, 515 (2001).

[17] Yusuke Nomura and Ryotaro Arita, "Ab initio downfolding for electron-phonon-coupled systems: Constrained density-functional perturbation theory," Phys. Rev. B **92**, 245108 (2015).
